# Supplementary material for: Silicon Nanowires as Anodes for Lithium-Ion Batteries: Full Cell Modeling
Source: arXiv:2401.16125 ancillary file (2024-01-29)
Supplement: Supplementary file 1 [file Supplementary_Information.pdf]

# Supporting Information: Silicon Nanowires as Anodes for Lithium-Ion Batteries: Full Cell Modeling

Franziska Kilchert,[†,‡] Max Schammer,[†,‡] Arnulf Latz,[†,‡,¶] and Birger Horstmann[*,†,‡,¶]

†*German Aerospace Center, Wilhelm-Runge-Straße 10, 89081 Ulm, Germany*

‡*Helmholtz Institute Ulm, Helmholtzstraße 11, 89081 Ulm, Germany*

¶*Universität Ulm, Albert-Einstein-Allee 47, 89081 Ulm, Germany*

E-mail: birger.horstmann@dlr.de

# Contents

S-1 Theory S-2

S-1.1 Ionic Liquid Electrolyte Theory . . . S-2

S-1.2 Silicon Nanowire Anode Theory . . . S-7

S-2 Parameterization S-12

S-2.1 Minimal Porosity Threshold . . . S-12

S-2.2 Ionic Liquid Electrolyte . . . S-12

S-2.3 Open Circuit Voltage Curves . . . S-12

S-2.4 Porosity and Active Mass Loading . . . S-13

S-2.5 Specific Surface Area . . . S-14

S-2.6 Rate Constant . . . S-14

S-3 Simulation Results S-15

S-3.1 Baseline Simulation . . . S-15

S-3.1.1 Cauchy Stress versus x-dimension . . . S-15

S-3.1.2 Tangential Component of Cauchy Stress . . . S-16

References S-19

# S-1 Theory

## S-1.1 Ionic Liquid Electrolyte Theory

To model the transport in the ionic liquid (IL) electrolyte we use our novel transport theory for highly concentrated electrolytes which is based on non-equilibrium thermodynamics as well as electromagnetic theory and mechanics.[S1] The transport equations are derived thermodynamically consistent from the free energy density and include convection which is a significant transport mechanism in solvent-free electrolytes. In this section, we summarize the transport theory for the

isothermal case ($T$ = const.). For a detailed derivation we refer the interested reader to Ref. S1. Since this section is focusing on the electrolyte only, we omit the superscript "e" here, *e.g.* for the concentration.

In the framework of rational thermodynamics it follows from the second law of thermodynamics that the entropy is not conserved. We use the entropy production rate $\mathcal{R}$ as measure for the deviation from thermodynamic equilibrium. Thus, $\mathcal{R}$ has to be strictly non-negative and includes contributions from internal friction (viscosity) and thermodynamic fluxes. The flux term $\mathcal{R}^{\text{flux}}$ comprises correlations between thermodynamic fluxes (electric current density $\mathbf{J}$, species flux densities $\mathbf{N}_\alpha$) and forces (electric potential $\Phi$, chemical potentials $\mu_\alpha$) and reads

$$\mathcal{R}^{\text{flux}} = -\mathbf{J}\nabla\Phi - \sum_{\alpha=1}^{N} \mathbf{N}_\alpha \nabla\mu_\alpha. \tag{S-1}$$

The model free energy density for bulk ionic liquid electrolytes has the following form,

$$\rho\varphi^{\text{H}} = \frac{\mathbf{DE}}{2} + \frac{K}{2}\left(1 - \sum_{\alpha=1}^{N} \nu_\alpha^0 c_\alpha\right)^2 + \bar{R}T \sum_{\alpha=1}^{N} c_\alpha \ln\frac{c_\alpha}{c} + \rho\varphi^{\text{H}}_{\text{int}}. \tag{S-2}$$

Here, the first term is the electrostatic energy density of polarizable media and contains the dielectric displacement $\mathbf{D}$ and the electric field $\mathbf{E}$. The second term comprises the energy of deformations and is defined relative to a stable reference configuration where the partial molar volumes take the value $\nu_\alpha^0$. $K$ is the bulk modulus and $c_\alpha$ the concentration of species $\alpha$. The third term contains the universal gas constant $\bar{R}$ and the temperature $T$. It represents the entropy of mixture for non-interacting systems. Finally, the last term comprises contributions from non-ideal interactions phenomenologically. Here, the deviation from ideal electrolytes can be included via activity coefficients. Variation of the free energy density yields the constitutive equations. For example, differentiating $\rho\varphi^{\text{H}}$ with respect to the concentration $c_\alpha$ yields the chemical potential $\mu_\alpha$,

$$\mu_\alpha = \frac{\partial\left(\rho\varphi^{\text{H}}\right)}{\partial c_\alpha}. \tag{S-3}$$

The total charge density $q = F \sum_{\alpha=1}^{N} z_\alpha c_\alpha$ is conserved and from charge continuity follows that

$$\mathbf{J} = F \sum_{\alpha=1}^{N} z_\alpha \mathbf{N}_\alpha, \tag{S-4}$$

where $F$ is the Faraday constant and $z_\alpha$ the charge number of species $\alpha$. Thus, we can express $\mathcal{R}^{\text{flux}}$ via the electrochemical potentials $\varphi_\alpha = \mu_\alpha + F z_\alpha \Phi$ as

$$\mathcal{R}^{\text{flux}} = -\sum_{\alpha=1}^{N} \mathbf{N}_\alpha \nabla \varphi_\alpha. \tag{S-5}$$

Due to certain constraints acting on the species flux densities, not all of them are independent. In the present center-of-mass (CM) reference frame, the flux densities are defined relative to the CM velocity $\mathbf{v} = \sum_{\alpha=1}^{N} \rho_\alpha \cdot \mathbf{v}_\alpha / \rho$ as

$$\mathbf{N}_\alpha = c_\alpha (\mathbf{v}_\alpha - \mathbf{v}). \tag{S-6}$$

Here, $\rho = \sum_{\alpha=1}^{N} \rho_\alpha = \sum_{\alpha=1}^{N} M_\alpha c_\alpha$ is the total mass density and $M_\alpha$ the molar mass of species $\alpha$. Thus, the following constraint on the species flux densities arises in the CM reference frame due to mass conservation,

$$\sum_{\alpha=1}^{N} M_\alpha \mathbf{N}_\alpha = 0. \tag{S-7}$$

This reduces the number of independent species and, thus, flux densities by one. We designate one species ($\alpha = 1$) and define reduced valences $\tilde{z}_\alpha$ and reduced chemical potentials $\tilde{\mu}_\alpha$,

$$\tilde{z}_\alpha = z_\alpha - \frac{M_\alpha}{M_1} z_1 \quad \text{and} \quad \tilde{\mu}_\alpha = \mu_\alpha - \frac{M_\alpha}{M_1} \mu_1. \tag{S-8}$$

With this, we get reduced electrochemical potentials $\tilde{\varphi}_\alpha = \tilde{\mu}_\alpha - F \tilde{z}_\alpha \Phi$ and the flux part of the entropy production rate takes the form

$$\mathcal{R}^{\text{flux}} = -\sum_{\alpha=2}^{N} \mathbf{N}_\alpha \nabla \tilde{\varphi}_\alpha. \tag{S-9}$$

We ensure a positive entropy production rate by using an Onsager approach to couple the thermodynamic fluxes and forces,

$$\mathbf{N}_\alpha = -\sum_{\beta=2}^{N} \mathcal{L}_{\alpha\beta} \nabla \tilde{\varphi}_\beta. \tag{S-10}$$

Here, $\mathcal{L}_{\alpha\beta}$ is the symmetric, semi-positive definite Onsager matrix. The macroscopic transport parameters follow directly from the Onsager coefficients in $\mathcal{L}_{\alpha\beta}$.

Applying charge continuity in the reduced form, $\mathbf{J} = \sum_{\alpha=2}^{N} F\tilde{z}_\alpha \mathbf{N}_\alpha$, leads to another reduction of the set of independent variables. We designate a second species ($\alpha = 2$) and define further reduced chemical potentials,

$$\tilde{\tilde{\mu}}_\alpha = \tilde{\mu}_\alpha - \frac{\tilde{z}_\alpha}{\tilde{z}_2} \tilde{\mu}_2. \tag{S-11}$$

From the Onsager approach we, thus, get the following expressions for the electric current density and the species flux densities,

$$\mathbf{J} = -\kappa \nabla \phi - \frac{\kappa}{F} \sum_{\beta=3}^{N} \frac{t_\beta}{\tilde{z}_\beta} \nabla \tilde{\tilde{\mu}}_\beta \tag{S-12}$$

$$\mathbf{N}_\alpha = \frac{t_\alpha}{F\tilde{z}_\alpha} \mathbf{J} - \sum_{\beta=3}^{N} D^{\mathrm{e}}_{\alpha\beta} \nabla \tilde{\tilde{\mu}}_\beta, \quad \alpha \geq 3. \tag{S-13}$$

Here, $\phi$ is an alternative form of the electric potential in the reduced description or chemo-electric potential,[S2,S3] $\phi = \Phi + \tilde{\mu}_2 / F\tilde{z}_2$. Furthermore, $\kappa$ is the conductivity, $t_\alpha$ the transference number in the reduced formalism and $D^{\mathrm{e}}_{\alpha\beta}$ the diffusion coefficient with respect to the reduced electrochemical potential. These transport parameters are all derived from the Onsager coefficients. Note that there exist only $N-1$ transference numbers in this reduced formalism and only $N-2$ are independent due to the normalization constraint $\sum_{\alpha=2}^{N} t_\alpha = 1$. The flux densities $\mathbf{N}_1$ and $\mathbf{N}_2$ are determined via the electric current density, eq. (S-4), and mass conservation, eq. (S-7).

From our model free energy density and together with the Euler equation for the volume,

$$\sum_{\alpha=1}^{N} c_\alpha \nu_\alpha = 1, \tag{S-14}$$

we also get an equation for the CM velocity,

$$\nabla \mathbf{v} = -\sum_{\alpha=1}^{N} \nu_\alpha \nabla \mathbf{N}_\alpha. \tag{S-15}$$

Also, from the Euler equation for the volume and the charge density we can determine the dependent concentrations $c_1$ and $c_2$. Via mass and charge conservation the number of independent species is reduced by two. From the Euler equation for the volume, eq. (S-14), follows directly for $c_1$

$$c_1 = \frac{1}{\nu_1}\left(1 - \nu_2 c_2 - \sum_{\alpha=3}^{\mathrm{N}} \nu_\alpha c_\alpha\right). \tag{S-16}$$

Using this expression together with charge conservation, $q = F\sum_{\alpha=1}^{\mathrm{N}} z_\alpha c_\alpha$, we can determine $c_2$

$$c_2 = \frac{z_1 - \nu_1 q/F}{\nu_2 z_1 - \nu_1 z_2} + \sum_{\alpha=3}^{\mathrm{N}} c_\alpha \frac{\nu_\alpha z_1 - \nu_1 z_\alpha}{\nu_1 z_2 - \nu_2 z_1}, \tag{S-17}$$

where $q$ is the charge density. Thus, in the electroneutral case ($q = 0$) the charge term vanishes.

Finally, we get the following closed set of isothermal transport equations including continuity equations for charge and concentration as well as the convection equation,

$$\frac{\partial q}{\partial t} = -\nabla \mathbf{J} - \nabla(q\mathbf{v}), \tag{S-18}$$

$$\frac{\partial c_\alpha}{\partial t} = -\nabla \mathbf{N}_\alpha - \nabla(c_\alpha \mathbf{v}), \quad \alpha \geq 3, \tag{S-19}$$

$$\nabla \mathbf{v} = -\frac{\tilde{\nu}_2}{F\tilde{z}_2}\nabla \mathbf{J} - \sum_{\alpha=3}^{N} \tilde{\tilde{\nu}}_\alpha \nabla \mathbf{N}_\alpha. \tag{S-20}$$

The Poisson equation couples the charge density and the electric potential via $q = -\epsilon_\mathrm{R}\epsilon_0 \Delta\Phi$, where $\epsilon_\mathrm{R}$ is the relative and $\epsilon_0$ the vacuum permittivity.

The final equations for modeling the electrolyte in the present battery cell are listed in table I in the main script. We assume electroneutrality ($q = 0$) in the bulk electrolyte and add source terms to account for the interplay with the electrodes. Furthermore, the equations are modified by porous electrode theory and limited to three species, see also sections II and II B. In table I and for the

simulations in this work, the anion is chosen as the first, the cation as the second and Li as the third species. However, the species order is freely selectable and this choice does not alter model results as long as it is kept consistent.[S1]

### S-1.2 Silicon Nanowire Anode Theory

In this section, we summarize the chemo-mechanically coupled model from Kolzenberg et al. that combines chemical expansion due to solid diffusion and mechanical deformations.[S4,S5] For a more detailed derivation of the theory see Refs. S4,S5. Note, that we omit the superscript "a" for anode in this section, *e.g.* for the concentration.

To avoid convective effects from the changing geometry the theory is established in the Lagrangian point of view. The Lagrangian description always refers to a fixed reference state of the system which in this case is the initial, pristine state of the nanowire at time $t = 0$ (subscript "0"). In this Lagrangian description the Si mass and volume are constant by definition. Thus, also the Si density $\rho_{\mathrm{Si},0}$ of the reference state stays constant, $\mathrm{d}\rho_{\mathrm{Si},0}/\mathrm{d}t = 0$.

A Si-mass-specific, intensive quantity $\psi_{\mathrm{Si}}$ can change with time due to a flux related to $\psi_{\mathrm{Si}}$ ($\mathbf{N}_{\psi,0}$) or the production of $\psi_{\mathrm{Si}}$ via a production rate $B_\psi$. This results in the following differential balance equation in the Lagrangian description,

$$\rho_{\mathrm{Si},0}\dot{\psi}_{\mathrm{Si}} = -\nabla_0 \mathbf{N}_{\psi,0} + \rho_{\mathrm{Si},0} B_\psi, \tag{S-21}$$

with the material derivative $\dot{\psi}_{\mathrm{Si}} = \partial\psi_{\mathrm{Si}}/\partial t + \mathbf{v}_{\mathrm{Si}}\nabla\psi_{\mathrm{Si}}$ where $\mathbf{v}_{\mathrm{Si}}$ is the center-of-mass velocity of the host material Si.

In the present case, Li is the only mobile species. Thus, based on eq. (S-21), we find for the mass or species balance

$$\dot{c}_{\mathrm{Li},0} = -\nabla_0 \mathbf{N}_{\mathrm{Li},0}. \tag{S-22}$$

Here, $c_{\mathrm{Li}}$ is the amount concentration and $\mathbf{N}_{\mathrm{Li}}$ the flux density of Li. We neglect species reaction rates.

The momentum density $p$ can change over time due to a momentum flux or body forces $\rho_{\mathrm{Si},0} b_{\mathrm{Si}}$ resulting in the momentum balance

$$\rho_{\mathrm{Si},0} \dot{p}_{\mathrm{Si}} = \nabla_0 \mathbf{P} + \rho_{\mathrm{Si},0} b_{\mathrm{Si}}. \tag{S-23}$$

Here, $\mathbf{P}$ is the first Piola-Kirchhoff stress tensor which is related to the more intuitive Cauchy stress tensor $\sigma$ via

$$\mathbf{P} = J \sigma \mathbf{F}^{-\mathrm{T}}, \tag{S-24}$$

with the deformation gradient $\mathbf{F}$ and its determinant $J = \det(\mathbf{F})$.

Together with the momentum balance, eq. (S-23), we get for the change in internal energy density $u_{\mathrm{Si}}$,

$$\rho_{\mathrm{Si},0} \dot{u}_{\mathrm{Si}} = \mathbf{P} : \dot{\mathbf{F}}. \tag{S-25}$$

Thus, the energy balance in terms of the Helmholtz free energy density $\varphi^{\mathrm{H}}_{\mathrm{Si}} = u_{\mathrm{Si}} - T S_{\mathrm{Si}}$ takes the form,

$$\rho_{\mathrm{Si},0} \dot{\varphi}^{\mathrm{H}}_{\mathrm{Si}} = \mathbf{P} : \dot{\mathbf{F}} - \rho_{\mathrm{Si},0} T \dot{S}_{\mathrm{Si}}, \tag{S-26}$$

with the entropy density $S_{\mathrm{Si}}$.

Adhering to the second law of thermodynamics, the entropy production rate has to be strictly non-negative ($\mathcal{R} \geq 0$). The isothermal balance for the entropy density states

$$\rho_{\mathrm{Si},0} T \dot{S}_{\mathrm{Si}} = -\nabla_0 T \mathbf{N}_{S,0} + \mathcal{R}, \tag{S-27}$$

with the entropy flux $\mathbf{N}_{S,0} = \mu_{\mathrm{Li}} \mathbf{N}_{\mathrm{Li},0} / T$. Thus,

$$\mathcal{R} = \mathbf{P} : \dot{\mathbf{F}} - \rho_{\mathrm{Si},0} \dot{\varphi}^{\mathrm{H}}_{\mathrm{Si}} + \nabla_0 \mu_{\mathrm{Li}} \mathbf{N}_{\mathrm{Li},0} \geq 0. \tag{S-28}$$

For our purpose of modeling a mobile species (Li) in an elastic material (Si), we can neglect electrical and thermal contributions to the free energy density. We assume that $\varphi^{\mathrm{H}}$ depends on the

Li concentration and the reversible deformation, $\varphi^{\mathrm{H}}(c_{\mathrm{Li},0}, \mathbf{C}_{\mathrm{rev}})$, where $\mathbf{C}_{\mathrm{rev}}$ is the right reversible Cauchy-Green tensor. Thus, the total time derivative takes the following form,

$$\begin{aligned}\rho_{\mathrm{Si},0}\dot{\varphi}^{\mathrm{H}}_{\mathrm{Si}} &= \rho_{\mathrm{Si},0}\frac{\partial \varphi^{\mathrm{H}}_{\mathrm{Si}}}{\partial c_{\mathrm{Li},0}}\dot{c}_{\mathrm{Li},0} + \rho_{\mathrm{Si},0}\frac{\partial \varphi^{\mathrm{H}}_{\mathrm{Si}}}{\partial \mathbf{C}_{\mathrm{rev}}}\dot{\mathbf{C}}_{\mathrm{rev}} \\ &= \mu_{\mathrm{Li}}\dot{c}_{\mathrm{Li},0} + \frac{1}{2}\mathbf{T}_{\mathrm{rev}} : \dot{\mathbf{C}}_{\mathrm{rev}}.\end{aligned} \tag{S-29}$$

Here, we make use of the definition of the chemical potential,

$$\mu_{\mathrm{Li}} = \rho_{\mathrm{Si},0}\frac{\partial \varphi^{\mathrm{H}}_{\mathrm{Si}}}{\partial c_{\mathrm{Li},0}}, \tag{S-30}$$

and identify the reversible second Piola-Kirchhoff stress tensor as

$$\mathbf{T}_{\mathrm{rev}} = 2\rho_{\mathrm{Si},0}\frac{\partial \varphi^{\mathrm{H}}_{\mathrm{Si}}}{\partial \mathbf{C}_{\mathrm{rev}}} = J\mathbf{F}^{-1}_{\mathrm{rev}}\sigma\mathbf{F}^{-\mathrm{T}}_{\mathrm{rev}}. \tag{S-31}$$

We do not account for plastic deformations. Thus, the entropy production rate reduces to

$$\mathcal{R} = -\mathbf{N}_{\mathrm{Li},0}\nabla_0\mu_{\mathrm{Li}} \geq 0. \tag{S-32}$$

The Onsager ansatz yields the Li flux density,

$$\mathbf{N}_{\mathrm{Li},0} = -\mathcal{M}_{\mathrm{Li}}\nabla_0\mu_{\mathrm{Li}}. \tag{S-33}$$

Here, $\mathcal{M}_{\mathrm{Li}}$ is the isotropic mobility of Li[S6] defined as

$$\mathcal{M}_{\mathrm{Li}} = \frac{D^{\mathrm{a}}_{\mathrm{Li}}c^{\max}_{\mathrm{Li},0}}{\bar{R}T}\theta_{\mathrm{Li}}(1-\theta_{\mathrm{Li}}), \tag{S-34}$$

where $D^{\mathrm{a}}_{\mathrm{Li}}$ is the solid diffusion coefficient of Li in Si and $\theta_{\mathrm{Li}} = c_{\mathrm{Li},0}/c^{\max}_{\mathrm{Li},0}$ is the dimensionless concentration or state of charge (SOC) with $c^{\max}_{\mathrm{Li},0}$ being the maximum possible concentration of Li in Si.

The chemical potential depends on the specific form of the model free energy. If we apply the model assumption from above and neglect electric, thermal and plastic effects, the deformation is completely reversible, $\mathbf{F} = \mathbf{F}_{\text{rev}}$. We divide the reversible deformation gradient into an elastic and a chemical contribution,

$$\mathbf{F}_{\text{rev}} = \mathbf{F}_{\text{elas}}\mathbf{F}_{\text{chem}}. \tag{S-35}$$

Thus, also the free energy density contains a chemical and mechanical (elastic) part,

$$\rho_{\text{Si},0}\varphi^{\text{H}}_{\text{Si}} = \rho_{\text{Si},0}\varphi^{\text{H}}_{\text{Si,chem}}(c_{\text{Li},0}) + \rho_{\text{Si},0}\varphi^{\text{H}}_{\text{Si,elas}}(c_{\text{Li},0}, \mathbf{F}_{\text{elas}}). \tag{S-36}$$

The chemical contribution is defined as

$$\rho_{\text{Si},0}\varphi^{\text{H}}_{\text{Si,chem}} = \bar{R}T c^{\max}_{\text{Li},0} \left(\theta_{\text{Li}} \ln(\theta_{\text{Li}}) + (1-\theta_{\text{Li}}) \ln(1-\theta_{\text{Li}})\right). \tag{S-37}$$

The elastic part has the form,

$$\rho_{\text{Si},0}\varphi^{\text{H}}_{\text{Si,elas}} = \frac{1}{2}\mathbf{E}_{\text{elas}} : \mathbb{C}\mathbf{E}_{\text{elas}} = \frac{1}{2}\mathbf{E}_{\text{elas}} : \mathbf{T}_{\text{rev}}, \tag{S-38}$$

where $\mathbf{E}_{\text{elas}}$ is the elastic deformation in the form of the Green-Lagrange strain tensor and $\mathbb{C}$ the elasticity tensor. The elastic deformation equals

$$\mathbf{E}_{\text{elas}} = \frac{1}{2}(\mathbf{C}_{\text{rev}} - \mathbf{C}_{\text{chem}}) = \frac{1}{2}\left(\mathbf{F}^{\text{T}}_{\text{rev}}\mathbf{F}_{\text{rev}} - \mathbf{F}^{\text{T}}_{\text{chem}}\mathbf{F}_{\text{chem}}\right), \tag{S-39}$$

which results in $\mathbf{T}_{\text{rev}} = \mathbb{C}\mathbf{E}_{\text{elas}}$ when calculating $\mathbf{T}_{\text{rev}}$ according to eq. (S-31). The elasticity tensor $\mathbb{C}$ can be written in Voigt notation and with symmetry consideration reduces to

$$\mathbb{C} = \frac{E}{(1+\nu)(1-2\nu)}\begin{pmatrix} 1-\nu & \nu & \nu \\ \nu & 1-\nu & \nu \\ \nu & \nu & 1-\nu \end{pmatrix}, \tag{S-40}$$

where $E$ is the elastic or Young's modulus of Si and $\nu$ the Poisson ratio.

The reversible, chemical deformation is assumed to be isotropic and the chemical deformation gradient comprises only the chemical deformation $\lambda_{\text{chem}}$,

$$\mathbf{F}_{\text{chem}} = \lambda_{\text{chem}} \cdot \mathbf{I}. \tag{S-41}$$

Here, $\mathbf{I}$ is the identity matrix. Thus, the determinant equals

$$J_{\text{chem}} = \lambda_{\text{chem}}^3 = 1 + \frac{\nu_{\text{Li}}^{\text{Si}}}{\nu_{0,\text{Si}}} 3.75\theta_{\text{Li}}, \tag{S-42}$$

with $\nu_{0,\text{Si}} = 10.96\times10^{-6}\,\text{m}^3\,\text{mol}^{-1}$ being the initial molar volume of Si and $\nu_{\text{Li}}^{\text{Si}} = 9\times10^{-6}\,\text{m}^3\,\text{mol}^{-1}$ the molar volume that Li occupies in Si alloys.[S7] The factor 3.75 stems from the highest lithiated phase of Si, which is $Li_{15}Si_4$ . Thus, the number of Li atoms per Si atom equals $3.75\theta_{\text{Li}}$.

In our case of modeling NWs, we assume a cylindrical geometry where the expansion in longitudinal direction (z, towards the separator) is hindered by the separator. The reversible deformation, thus, has the form

$$\mathbf{F}_{\text{rev}} = \begin{pmatrix} \lambda_{\text{r}} & 0 & 0 \\ 0 & \lambda_{\phi} & 0 \\ 0 & 0 & \lambda_{\text{chem}} \end{pmatrix}, \tag{S-43}$$

where the radial component of the deformation is defined as $\lambda_{\text{r}} = \partial r/\partial R_0$ and the angular part $\lambda_{\phi} = r/R_0$. Here, $r$ is the varying, current radius of the NW while $R_0$ is the initial radius. With all this, the chemical potential according to eq. (S-30) equals,

$$\mu_{\text{Li}} = \bar{R}T \ln\left(\frac{\theta_{\text{Li}}}{1-\theta_{\text{Li}}}\right) - \frac{3.75\nu_{\text{Li}}^{\text{Si}}}{3\nu_{0,\text{Si}} c_{\text{Li},0}^{\text{max}} \lambda_{\text{chem}}} \text{tr}\left(\mathbf{T}_{\text{rev}}\right). \tag{S-44}$$

Thus, we can solve the balance eqs. (S-22) and (S-23) where we neglect inertial ($\dot{p}_{\text{Si}}$) and body ($b_{\text{Si}}$) forces. The final equations for modeling the anode in their specific form in cylindrical coordinates are listed in table I in the main script.

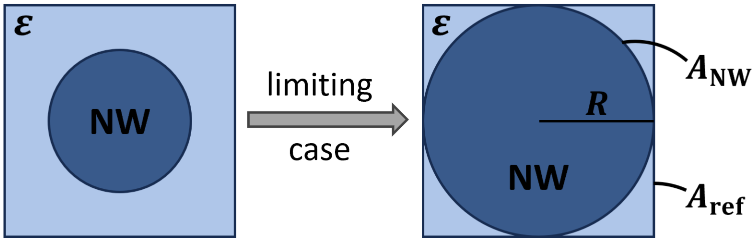


Figure S1: Schematic of the geometry for the anode porosity threshold.

# S-2 Parameterization

## S-2.1 Minimal Porosity Threshold

Due to the expansion of the Si NWs on the anode side, a cut-off condition for the minimal porosity of the anode has to be set. When the NWs reach a certain diameter they start to touch (see the schematic fig. S1), which creates large stresses in the anode and can block electrolyte diffusion paths. The threshold value is solely depending on the geometry of the anode. Since we model the NWs as cylinders the porosity limit can be determined from the NW cross section. We assume a primitive cubic lattice arrangement of the NWs. In the limiting case, the residual pore space $\varepsilon$ is calculated by dividing the NW cross sectional area $A_{\mathrm{NW}} = \pi R^2$ by the reference cross sectional area $A_{\mathrm{ref}} = 4R^2$. Thus,

$$\varepsilon = 1 - \frac{A_{\mathrm{NW}}}{A_{\mathrm{ref}}} = 1 - \frac{\pi}{4} = 21.46\%. \qquad \text{(S-45)}$$

Therefore, we set the porosity threshold on the anode side to 22%.

## S-2.2 Ionic Liquid Electrolyte

As electrolyte we use the IL + Li-salt mixture (0.4)LiFSI(0.6)Pyr12O1FSI. Here, FSI is the chemical acronym for bis(fluorosulfonyl)imide and Pyr12O1 stands for 1-methoxyethyl-1-methylpyrrolidinium.

## S-2.3 Open Circuit Voltage Curves

Open circuit voltage (OCV) curves $U_0^{\mathrm{s}}(\theta_{\mathrm{Li}}^{\mathrm{s}})$ are necessary input parameters for our physics-based full cell simulations. Here, $\theta_{\mathrm{Li}}^{\mathrm{s}}$ is the state of charge (SOC) of the respective electrode. For the

NMC111 cathode material we take the OCV curve from Ref. S8:

$$U_0^{\mathrm{NMC}}\left(\theta_{\mathrm{Li}}^{\mathrm{NMC}}\right) = 7.9760 - 5.5419 \cdot \theta_{\mathrm{Li}}^{\mathrm{NMC}} + 5.2824 \cdot \left(\theta_{\mathrm{Li}}^{\mathrm{NMC}}\right)^{1.07} - 1.0556 \cdot 10^{-4} \cdot \exp\left(124.7407 \cdot \theta_{\mathrm{Li}}^{\mathrm{NMC}} - 114.2593\right) - 4.0446 \cdot \left(\theta_{\mathrm{Li}}^{\mathrm{NMC}}\right)^{0.0766}. \quad \text{(S-46)}$$

For the silicon anode, we apply a fit to the GITT measurement data from Ref. S9:

$$U_0^{\mathrm{Si}}\left(\theta_{\mathrm{Li}}^{\mathrm{Si}}\right) = [-2.5463 \cdot \left(\theta_{\mathrm{Li}}^{\mathrm{Si}}\right)^8 + 10.2358 \cdot \left(\theta_{\mathrm{Li}}^{\mathrm{Si}}\right)^7 - 24.3297 \cdot \left(\theta_{\mathrm{Li}}^{\mathrm{Si}}\right)^6 + 33.6197 \cdot \left(\theta_{\mathrm{Li}}^{\mathrm{Si}}\right)^5 - 24.7655 \cdot \left(\theta_{\mathrm{Li}}^{\mathrm{Si}}\right)^4 + 9.2289 \cdot \left(\theta_{\mathrm{Li}}^{\mathrm{Si}}\right)^3 - 1.9587 \cdot \left(\theta_{\mathrm{Li}}^{\mathrm{Si}}\right)^2 + 0.5586 \cdot \theta_{\mathrm{Li}}^{\mathrm{Si}} + 0.0127]/\left(\theta_{\mathrm{Li}}^{\mathrm{Si}} + 0.01\right). \quad \text{(S-47)}$$

Note that this fit is an averaging of the lithiation and delithiation curves.

## S-2.4 Porosity and Active Mass Loading

For a given active mass loading of an electrode $a^{\mathrm{s}}$ the porosity of this electrode can be estimated. We show the calculation for our Si NW electrodes where we assume that the NWs consist of pure amorphous Si. We approximate the porosity by dividing the volume that the NWs occupy ($V_{\mathrm{NWs}}$) by the total volume of the anode ($V^{\mathrm{a}}$). The volume of the NWs is determined via $V_{\mathrm{NWs}} = A^{\mathrm{a}} a^{\mathrm{a}} / \rho_{\mathrm{Si}}$ whereas the total volume of the anode equals $V^{\mathrm{a}} = A^{\mathrm{a}} L^{\mathrm{a}}$. Thus, the base area of the anode $A^{\mathrm{a}}$ cancels out,

$$\varepsilon^{\mathrm{a}} = 1 - \frac{V_{\mathrm{NWs}}}{V^{\mathrm{a}}} = 1 - \frac{a^{\mathrm{a}}}{\rho_{\mathrm{Si}} L^{\mathrm{a}}}. \quad \text{(S-48)}$$

Vice versa, the active mass loading of the Si NW anode can be calculated from the porosity by rearranging the above equation,

$$a^{\mathrm{a}} = (1 - \varepsilon^{\mathrm{a}}) \rho_{\mathrm{Si}} L^{\mathrm{a}}. \quad \text{(S-49)}$$

## S-2.5 Specific Surface Area

The specific surface area of the electrodes $A^{\mathrm{s}}_{\mathrm{spec}}$ is the electrode surface area per volume ($\mathrm{m}^2\,\mathrm{m}^{-3}$) in contact with the electrolyte. It enters the electrolyte transport equations via the source terms and influences how much Li is transported. We can estimate $A^{\mathrm{s}}_{\mathrm{spec}}$ from the geometry of the electrodes by dividing the surface area of the particles/cylinders by their volume. The porosity accounts for the volume-averaging from porous electrode theory. For the spherical cathode particles we, thus, get,

$$A^{\mathrm{c}}_{\mathrm{spec}} = \frac{A_{\mathrm{sphere}}}{V_{\mathrm{sphere}}} \cdot (1 - \varepsilon^{\mathrm{c}}) = \frac{3}{R^{\mathrm{c}}} \cdot (1 - \varepsilon^{\mathrm{c}})\,. \tag{S-50}$$

On the anode side, we approximate the NWs with cylinders. For the calculation of $A^{\mathrm{a}}_{\mathrm{spec}}$ we neglect the circular bases of the cylinder and assume transport is only happening through the lateral area ($A^{\mathrm{lateral}}_{\mathrm{cylin}} = 2\pi R^{\mathrm{a}} L^{\mathrm{a}}$). With this, we get,

$$A^{\mathrm{a}}_{\mathrm{spec}} = \frac{A^{\mathrm{lateral}}_{\mathrm{cylin}}}{V_{\mathrm{cylin}}} \cdot (1 - \varepsilon^{\mathrm{a}}) = \frac{2}{R^{\mathrm{a}}} \cdot (1 - \varepsilon^{\mathrm{a}})\,. \tag{S-51}$$

## S-2.6 Rate Constant

Rate constants in the Butler-Volmer-expression are usually given in terms of $\mathrm{m}^{2.5}\mathrm{mol}^{-0.5}\mathrm{s}^{-1}$ since the exchange current density is often written in terms of concentration. Here, we use the SOC instead. Thus, the rate constant $k^{\mathrm{s}}$ has the unit $\mathrm{mol\,m^{-2}\,s^{-1}}$ and can be calculated from the literature values $k^{\mathrm{s}}_{\mathrm{lit}}$ via

$$k^{\mathrm{s}} = k^{\mathrm{s}}_{\mathrm{lit}} \cdot c^{\mathrm{max,s}}_{\mathrm{Li}} \cdot \sqrt{c^{\mathrm{e}}_{\mathrm{Li,0}}}. \tag{S-52}$$

We use literature values from Ref. S10 and S11 for anode and cathode, respectively.

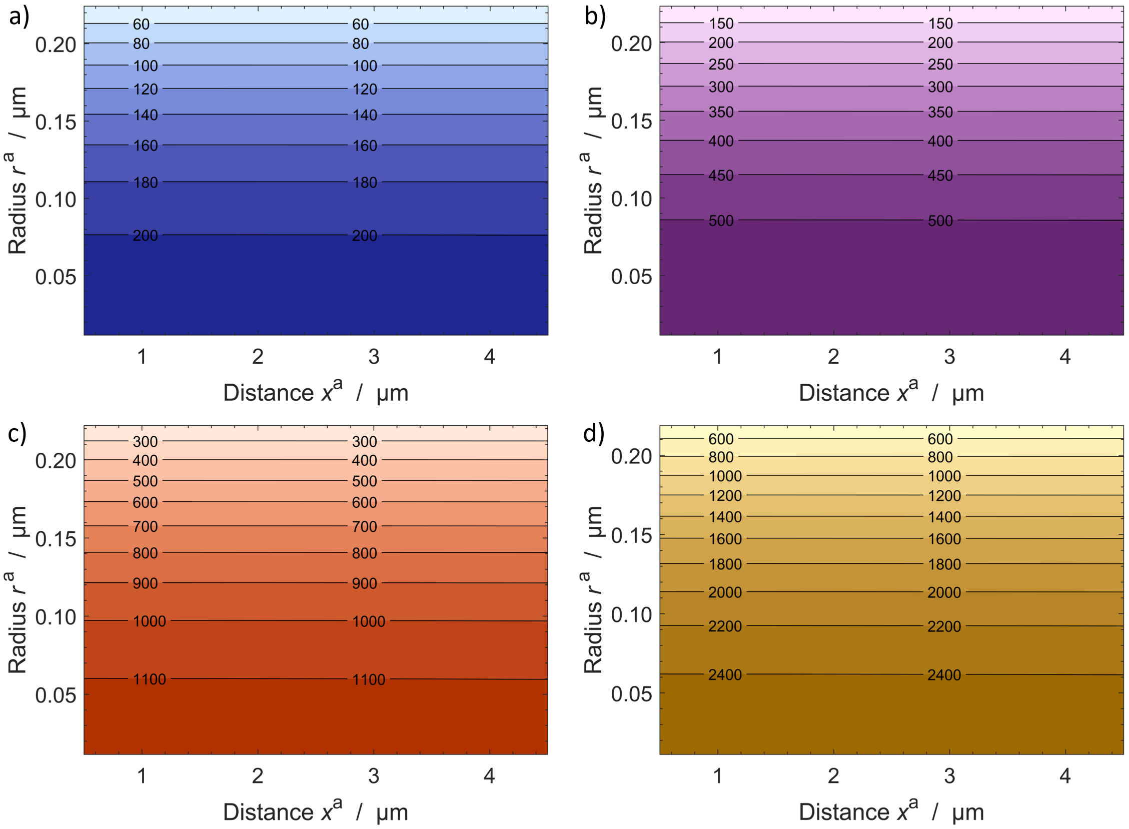


Figure S2: Spatially resolved radial component of the Cauchy stress (in MPa) at the end of charge after charging with a) C/50, b) C/20, c) C/10 and d) C/5.

# S-3 Simulation Results

## S-3.1 Baseline Simulation

### S-3.1.1 Cauchy Stress versus x-dimension

Figure S2 depicts the radial component of the Cauchy stress spatially resolved for every voxel in $x$- and $r$-direction. The figures a) to d) show the stress at the end of charge after charging with the for different C-rates C/50 to C/5. In all four cases there is no stress gradient visible along the $x$-coordinate. This indicates that the Li-ion transport in the electrolyte is fast enough to supply enough Li to the anode such that the NWs are lithiated evenly. For this reason, figs. 5 and 6 and figs. S3 and S4 are all depicted for only one voxel in $x$-direction, namely the one closest to the separator ($x^a$ = 4.5 µm). The observed gradient in the $r$-dimension is in accordance to the findings

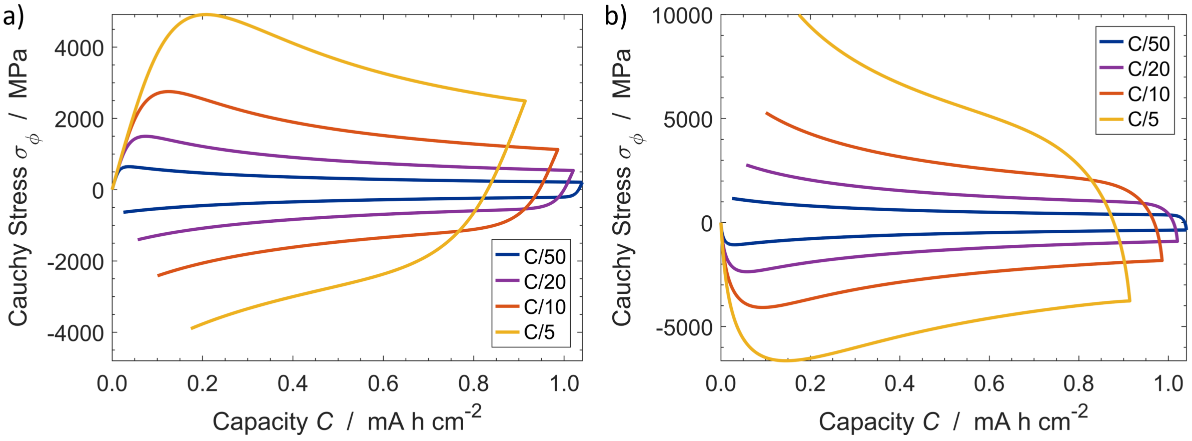


Figure S3: Evolution of the tangential component of the Cauchy stress a) near the center of the Si NWs and b) near the edge of the NWs over one charge-discharge cycle for different C-rates.

of fig. 6. In the middle of the NW the largest compressive stresses occur whereas to the edge of the NW the stress decreases. For the radial component the boundary condition of the stress is zero at the edge of the NWs.

### S-3.1.2 Tangential Component of Cauchy Stress

Figures S3 and S4 show the tangential component of the Cauchy stress. In fig. S3 a) this Cauchy stress component is plotted against the capacity for the four different C-rates C/50 to C/5 at the radial position $r_1$ near the center of the NW and in b) at the radial position $r_{10}$ near the edge of the NW. In contrast to the radial component, the tangential Cauchy stress has no zero stress boundary condition. Thus, we see that the tangential stress is actually largest near the edge of the NWs. Otherwise the curve shape is very similar to the one of the radial component and can be explained by the concentration gradients and the Eulerian perspective as outlined in the main script (see section III A). Over the course of the radial dimension the tangential Cauchy stress switches sign from compressive to tensile during charging and vice versa during discharging. This behaviour is also visible in the following fig. S4.

In fig. S4 a) the evolution of the tangential component of the Cauchy stress within the NW is shown versus cell capacity for three different radial positions within the NW (from $r_1$ in the center to $r_{10}$ near the edge). For visible clarity less curves are depicted in comparison to fig. 6 a). Fig-

ure S4 b) shows the tangential component of the Cauchy stress versus the NW radius for various times (corresponding to different states of charge (SOC) of the anode) during one full cycle. In both representations the change over the $r$-dimension from compressive (/tensile) to tensile (/compressive) stress during charging (/discharging) is clearly visible. Furthermore, the stress direction switches over the course of one cycle. These results are again in very good agreement with the observations for spherical Si particles presented in Ref. S5 (see, especially, Fig. 7 there).

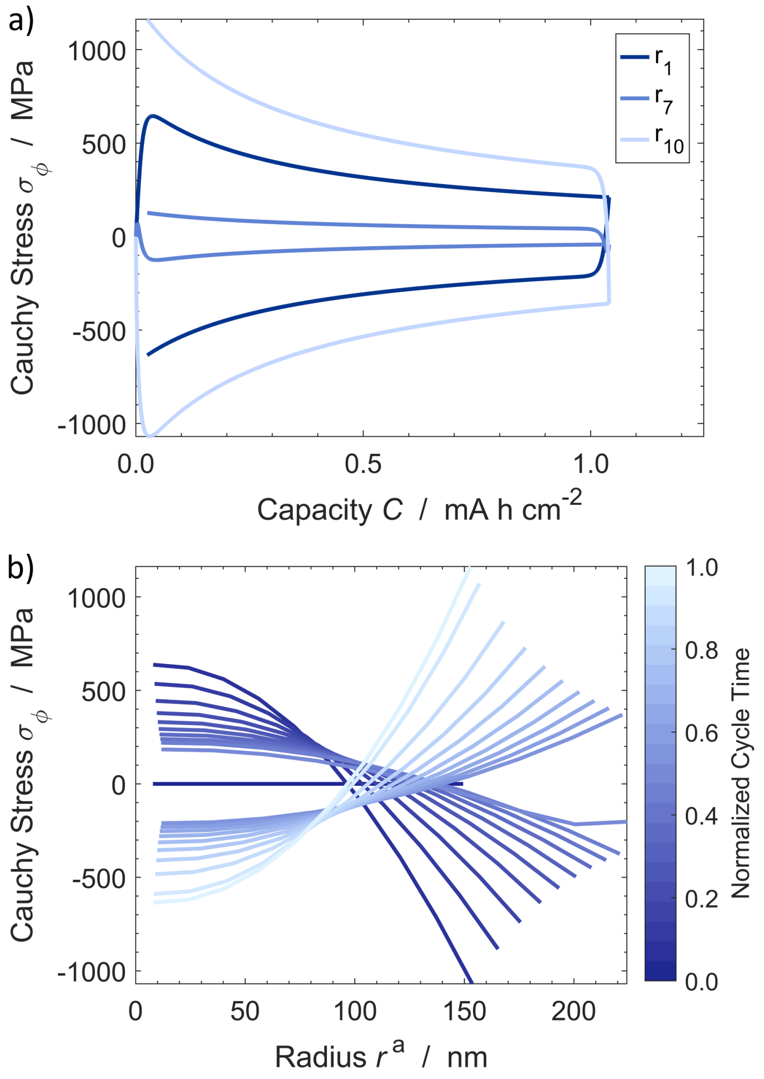


Figure S4: Evolution of the tangential component of the Cauchy stress within the NW shown a) versus cell capacity for different radial positions within the NW (from $r_1$ in the center to $r_{10}$ near the edge) and b) versus the NW radius for various times (corresponding to different anode SOCs) during one full cycle.

# References


(S1) Schammer, M.; Horstmann, B.; Latz, A. Theory of Transport in Highly Concentrated Electrolytes. *Journal of the Electrochemical Society* **2021**, *168*, 026511.

(S2) Newman, J.; Thomas-Alyea, K. E. *Electrochemical systems*; John Wiley & Sons, 2012.

(S3) Latz, A.; Zausch, J. Multiscale modeling of lithium ion batteries: thermal aspects. *Beilstein Journal of Nanotechnology* **2015**, *6*, 987–1007.

(S4) Castelli, G. F.; von Kolzenberg, L.; Horstmann, B.; Latz, A.; Dörfler, W. Efficient Simulation of Chemical-Mechanical Coupling in Battery Active Particles. *Energy Technology* **2021**, *9*, 2000835.

(S5) von Kolzenberg, L.; Latz, A.; Horstmann, B. Chemo-Mechanical Model of SEI Growth on Silicon Electrode Particles. *Batteries & Supercaps* **2022**, *5*.

(S6) Leo, C. V. D.; Rejovitzky, E.; Anand, L. A Cahn–Hilliard-type phase-field theory for species diffusion coupled with large elastic deformations: Application to phase-separating Li-ion electrode materials. *Journal of the Mechanics and Physics of Solids* **2014**, *70*, 1–29.

(S7) Obrovac, M. N.; Christensen, L.; Le, D. B.; Dahn, J. R. Alloy Design for Lithium-Ion Battery Anodes. *Journal of The Electrochemical Society* **2007**, *154*, A849.

(S8) Danner, T.; Singh, M.; Hein, S.; Kaiser, J.; Hahn, H.; Latz, A. Thick electrodes for Li-ion batteries: A model based analysis. *Journal of Power Sources* **2016**, *334*, 191–201.

(S9) Pan, K.; Zou, F.; Canova, M.; Zhu, Y.; Kim, J.-H. Systematic electrochemical characterizations of Si and SiO anodes for high-capacity Li-Ion batteries. *Journal of Power Sources* **2019**, *413*, 20–28.

(S10) Verma, A.; Franco, A. A.; Mukherjee, P. P. Mechanistic Elucidation of Si Particle Morphology on Electrode Performance. *Journal of The Electrochemical Society* **2019**, *166*, A3852–A3860.

(S11) Smekens, J.; Paulsen, J.; Yang, W.; Omar, N.; Deconinck, J.; Hubin, A.; Mierlo, J. V. A Modified Multiphysics model for Lithium-Ion batteries with a LixNi1/3Mn1/3Co1/3O2 electrode. *Electrochimica Acta* **2015**, *174*, 615–624.
